# Supplementary material for: Strong and selective magnon-phonon coupling in van der Waals antiferromagnet CoPS$_3$
Source: arXiv:2508.07412 source file (2025-08-10)
Supplement: Supplementary file 1 [file CoPS3_Magnon_SM.pdf]

# Strong and selective magnon-phonon coupling in van der Waals antiferromagnet $CoPS_3$

Dipankar Jana,[1,2,*] Diana Vaclavkova,[1] Rajesh Kumar Ulaganathan,[3] Raman Sankar,[3] Milan Orlita,[1,4] Clement Faugeras,[1] Maciej Koperski,[2,5] M. E. Zhitomirsky,[6,7] and Marek Potemski[1,8,9,†]

[1]*Laboratoire National des Champs Magnétiques Intenses, LNCMI-EMFL, CNRS UPR3228, Univ. Grenoble Alpes, Univ. Toulouse, Univ. Toulouse 3, INSA-T, Grenoble and Toulouse, France*
[2]*Institute for Functional Intelligent Materials, National University of Singapore, 117544, Singapore*
[3]*Institute of Physics, Academia Sinica, Taipei 10617, Taiwan*
[4]*Institute of Physics, Charles University, Ke Karlovu 5, Prague, 121 16, Czech Republic*
[5]*Department of Materials Science and Engineering, National University of Singapore, 117575, Singapore*
[6]*Universit´e Grenoble Alpes, CEA, Grenoble INP, IRIG, Pheliqs, 38000 Grenoble, France*
[7]*Institut Laue-Langevin, F-38042 Grenoble Cedex 9, France*
[8]*CENTERA, CEZAMAT, Warsaw University of Technology, 02-822 Warsaw, Poland*
[9]*Institute of High Pressure Physics, PAS, 01-142 Warsaw, Poland*

* jana.d02@nus.edu.sg
† marek.potemski@lncmi.cnrs.fr

## I. TEMPERATURE AND POLARIZATION-RESOLVED RAMAN SCATTERING RESPONSE OF $CoPS_3$

Raman scattering spectroscopy is a powerful technique for probing magnetic phase transitions and identifying magnon gap excitations distinct from phonon modes. Figure S1a presents the unpolarized Raman scattering spectra over a broad spectral range at selected temperatures. At room temperature, Several $E_g$ and $A_g$ phonon modes are observed, with the low frequency modes attributed to the vibrations of $Co^{2+}$ ions [S1]. As the temperature decreases, the phonon modes intensify and a broad spectral feature related to the two-magnon (2M) continuum emerges at around 350 $cm^{-1}$. It exists even above the Néel temperature due to the persistent short-range magnetic order. Additionally, the phonon mode($P_{2,3}$) near 150 $cm^{-1}$ splits into two components upon cooling, a behavior linked to the magnetostriction effect [S1]. However, our measurements reveal the emergence of two additional weak-intensity peaks (107 $cm^{-1}$ and 187 $cm^{-1}$), which we identify as signatures of magnon gap excitations. In the main text, we demonstrate that the 150 $cm^{-1}$ phonon splitting arises mainly due to the strong and selective coupling with magnon modes. Linear polarization–resolved Raman scattering measurements, as shown in Fig. S1b, reveal that the coupled magnon-like modes ($M_1'$ and $M_2'$) and phonon-like modes ($P_1'$, $P_2'$, and $P_3'$) exhibit strong sensitivity to the orientation of the laser polarization. The $M_1'$ and $P_3'$ modes emerge under cross-linear polarization, while $M_2'$, $P_1'$, and $P_2'$ modes are prominent in the co-linear polarization. This polarization dependence enables precise determination of the coupled mode's energy, even when spectral features broaden and overlap at higher temperatures, as illustrated in **Fig. 5b** of the main manuscript.

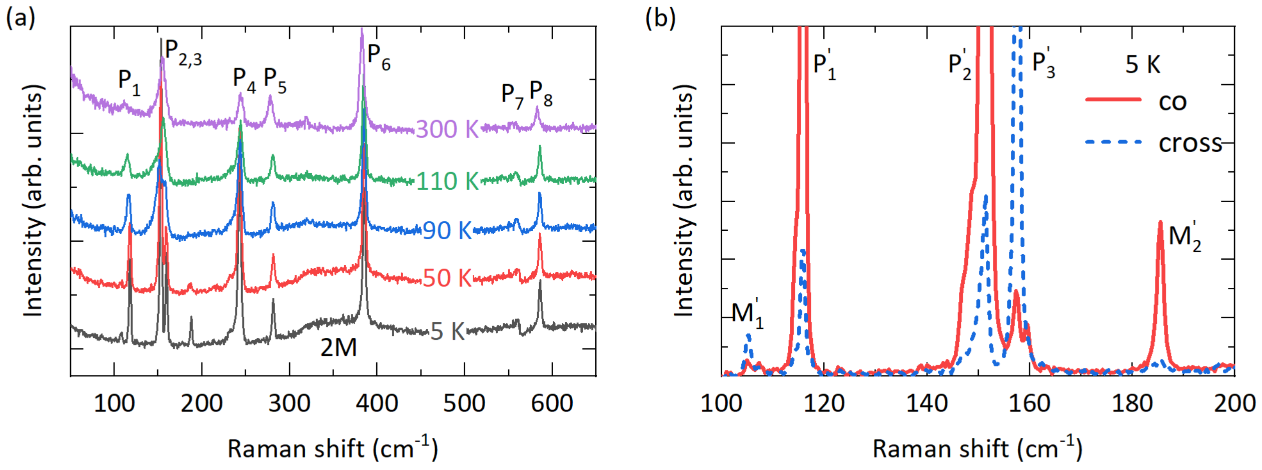


FIG. S1. (a) Raman scattering spectra of $CoPS_3$ in the wide spectral range measured at selected temperatures. $P_1$ to $P_8$ correspond to the phonon modes, while the two-magnon continuum mode is labeled as 2M. (b) Linear polarization-resolved Raman scattering spectra at 5 K. The magnon-like modes are marked as $M_i'$ while the phonon-like modes are marked as $P_i'$.

## II. RAMAN SCATTERING RESPONSE OF $CoPS_3$ AS A FUNCTION OF MAGNETIC FIELD

In the absence of magnetic field–induced structural modifications, phonon modes remain largely unaffected by an external magnetic field. In contrast, magnon modes exhibit characteristic field-dependent behavior that depends on the spin orientation relative to the magnetic field. Since the crystallographic axes were not determined experimentally, the magnetic field was applied along a chosen edge of the sample, which was assumed to correspond to a specific crystallographic—and thus magnetic—axis. The Raman scattering spectra measured as a function of the in-plane magnetic field are shown in Fig. S2 in the form of a false color map for different crystallographic orientations. Among these, the configurations displayed in Fig. S2a and S2d exhibit markedly contrasting magnetic field dependence of the coupled modes, and are therefore considered for detailed analysis in the main manuscript (**Fig. 2a, Fig. 3, and Fig. 4**). Further, the theoretical modeling of the main manuscript suggests that the field directions in Figs. S2a and S2d correspond approximately to magnetic fields applied along the crystallographic *a*- and *c*-axes, respectively. In Fig. S2b, a splitting of the $M_2^{'}$ mode is observed, which may result from the stacking of multiple domains with different orientations of magnetic x-axis under the excitation laser spot.

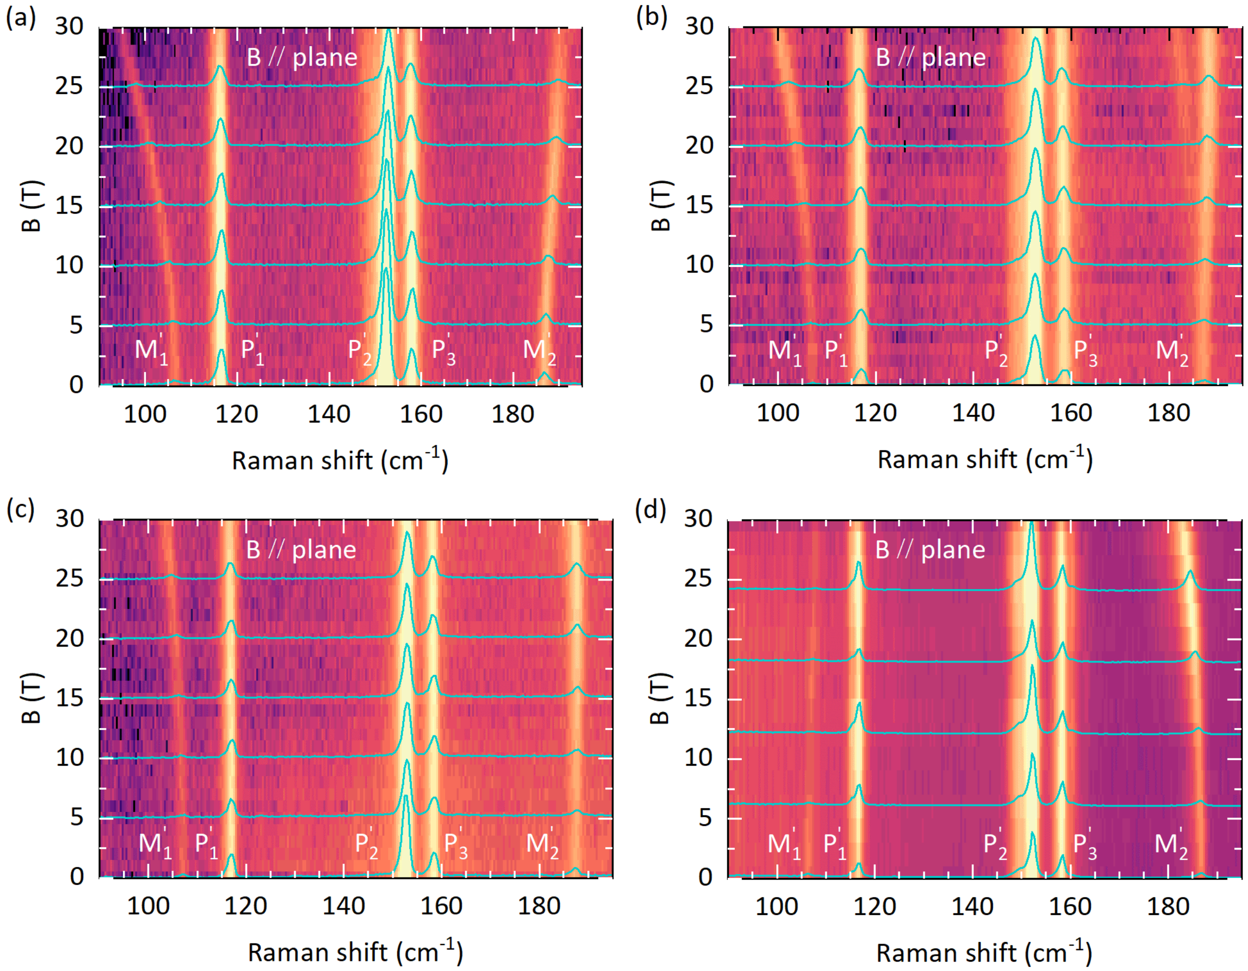


FIG. S2. (a)-(d) False color map of low-temperature (5 K) Raman scattering of $CoPS_3$ as a function of the magnetic field applied along different in-plane directions of the crystal. A few representative scattering spectra, measured at different magnetic field strengths, are also plotted. The magnon-like modes are marked as $M_i^{'}$ while the phonon-like modes are marked as $P_i^{'}$.

The application of an out-of-plane magnetic field is relatively straightforward. Fig. S3a shows the false color map of the low-temperature Raman scattering spectra of $CoPS_3$ as a function of magnetic field applied perpendicular to the sample plane. As reported in Ref. [S2], the spins in $CoPS_3$ are canted by 10° from the *a*-axis, toward the *c*-axis. Consequently, the applied magnetic field is not strictly orthogonal to the spin orientation. The extracted peak positions of the coupled magnon modes ($M_1^{'}$, $M_2^{'}$) are shown in **Fig. 4** of the main manuscript. are also shown in the same plot. Both the coupled magnon modes and the bare magnon modes($M_1$, $M_2$), as obtained by solving **Eq. 2** of the main manuscript, exhibit a linear dependence in the $B^2$ vs Energy$^2$ plot. The slopes are extracted to be slope ($M_1$) = 0.35 $cm^{-2}T^{-2}$ and slope ($M_2$) = 0.86 $cm^{-2}T^{-2}$ for the $M_1$ and $M_2$ modes respectively.

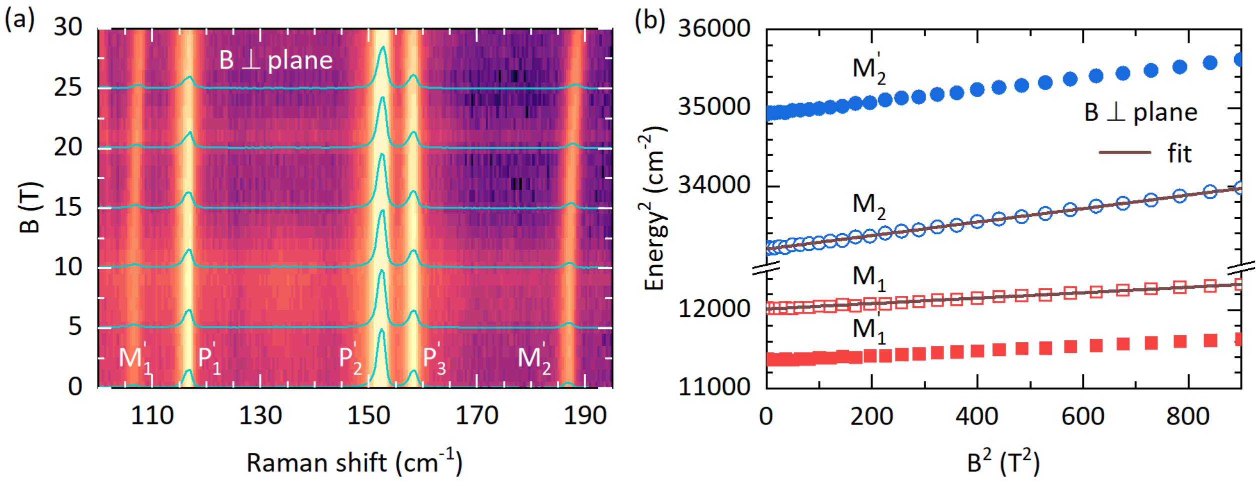


FIG. S3. (a) False color map of Raman scattering of $CoPS_3$ at 5 K measured as a function of the magnetic field applied perpendicular to the sample plane. A few representative scattering spectra, at 5 T intervals, are also plotted. The coupled magnon-like modes are labeled as $M_i^{'}$ while the phonon-like modes are labeled as $P_i^{'}$. (b) Peak energies of coupled magnon-like modes and the corresponding bare magnon modes ($M_1$ and $M_2$) are shown by solid and open symbols, respectively, in the $B^2$ vs Energy$^2$ plot. Solid lines display the linear fit of the magnetic field dependence of bare $M_1$ and $M_2$ modes.

## III. ESTIMATION OF MAGNON-PHONON COUPLING CONSTANTS

In this section, we outline the method used to estimate the bare manon and phonon energies and their coupling constants using **Eq. 2** of the main manuscript. Assuming selective coupling between the magnon and phonon modes, **Eq. 2** can be decomposed into two separate equations,

$$H_{3\times3} = \begin{bmatrix} \omega_{M1} & \delta_1 & \delta_2 \\ \delta_1 & \omega_{P1} & 0 \\ \delta_2 & 0 & \omega_{P3} \end{bmatrix} \qquad and \qquad H_{2\times2} = \begin{bmatrix} \omega_{M2} & \delta_3 \\ \delta_3 & \omega_{P2} \end{bmatrix} \tag{S1}$$

In each of these equations, the number of constraints (i.e., equations) is one fewer than the number of observables (i.e., unknown parameters). Consequently, the observables cannot be uniquely determined from a single set of coupled modes (e.g., the coupled mode energies at $B = 0\ T$). An additional constraint is therefore required, which can be obtained either from the magnetic field dependence of the coupled modes or by analyzing another set of coupled modes at a different temperature or magnetic field. However, the precise magnetic field dependence of the magnon modes is not known in our case, as the magnetic field was not aligned with any specific crystallographic direction in the experimental configuration. Thus, we adopt the second approach and estimate the coupling constants using the magnetic field–dependent data shown in **Fig. 3** (corresponding to the color plot in **Fig. 2a**) of the main manuscript. The resulting values of the coupling constants ($\delta_2$ and $\delta_3$), obtained via this two-dataset approach, are shown in Fig. S4. For instance, data points on the red curves correspond to calculations using one set of parameters at $B = 0$ T and a second set at magnetic fields above $B = 14$ T. The individual curves represent estimations where the first set of parameters is taken at magnetic field strengths ranging from $B = 0$ T to $B = 7$ T, in 1 T increments. In these calculations, the bare phonon energies are assumed to be field-independent. As expected, the uncertainty increases when the two datasets correspond to nearby field values, where the differences in the coupled mode energies are small. The average values of the estimated coupling constants are reported in the main manuscript. The corresponding bare mode energies and their magnetic field dependencies are also presented in **Fig. 3** of the main manuscript. For other cases involving magnetic field or temperature variations, the coupled magnon mode energies ($M_1'$, $M_2'$) and the averaged coupling constants are used to simulate the coupled phonon mode energies ($P_1'$, $P_2'$, and $P_3'$), which are plotted as solid lines in **Fig. 4b** of the main manuscript.

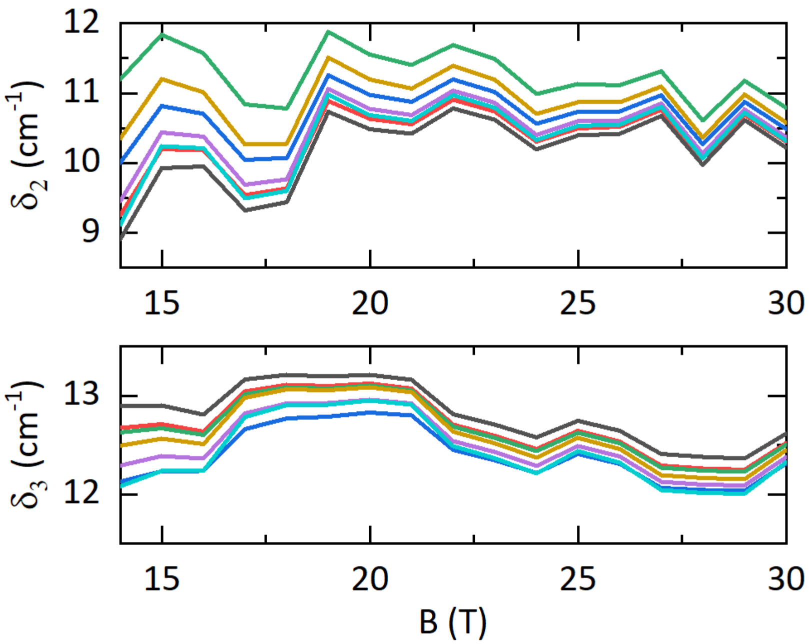


FIG. S4. Coupling constant estimated by considering a two-dataset approach. Each point on a line is obtained by taking one data set at a low field point and the second data set from 14 T to 30 T, while the individual line plots are for the first data set taken from seven low-field points (0 T to 7 T with 1 T step).

## IV. RAMAN SCATTERING RESPONSE OF $CoPS_3$ AS A FUNCTION OF TEMPERATURE

The same coupling coefficients and bare phonon energies were employed to reproduce the temperature dependence of the coupled modes. Figure S5a shows the calculated temperature evolution of the bare magnon and phonon mode energies (solid lines), derived using **Eq. 2** of the main manuscript, along with the experimentally observed coupled modes. As shown in Fig. S5b, the bare magnon energies follow a characteristic $T^{3.5}$ dependence. The extrapolated temperature dependence of both bare and coupled modes up to 90K is presented in **Fig. 5a** of the main manuscript. The simulation predicts a splitting of approximately 1 $cm^{-1}$ between the bare phonon modes ($P_2$ and $P_3$), whereas they appear degenerate in the paramagnetic phase, as indicated by the dashed line in Fig. S5a. This discrepancy points to additional effects, such as magnetostriction or coupling to a two-magnon continuum. Furthermore, a slight deviation is observed between the simulated and experimentally extracted bare phonon energies, implying that the phonon modes exhibit an intrinsic temperature dependence not fully captured by our model. Similar temperature-dependent behavior is also evident in other phonon modes, as shown in Fig. S5c

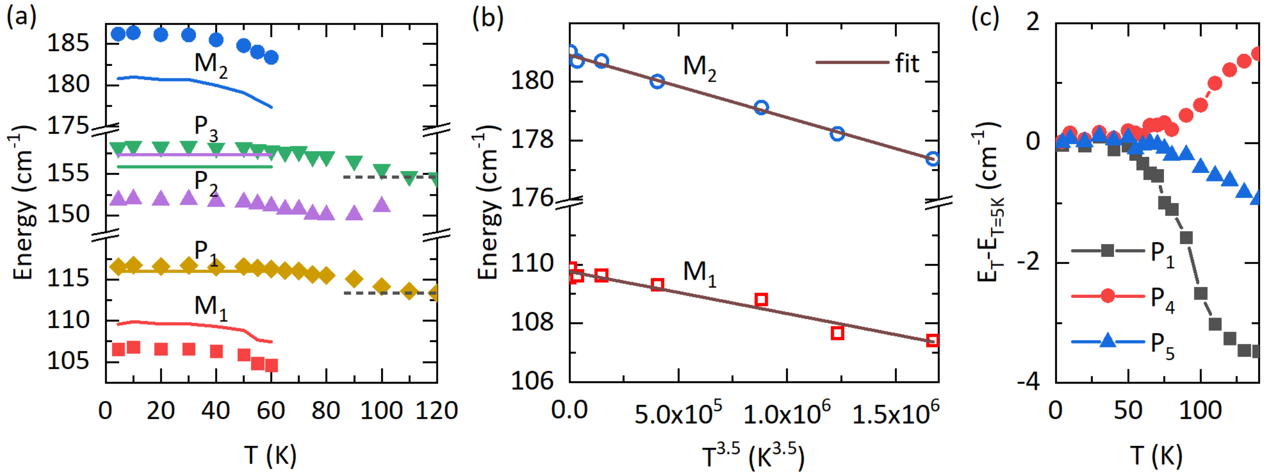


FIG. S5. (a) peak energies of the coupled (solid symbols) and bare (solid line) magnon and phonon modes as a function of temperature. The dashed black line corresponds to the phonon mode energies in the paramagnetic phase. (b) Bare magnon modes as a function of temperature following $T^{3.5}$ dependence. (c) Temperature dependence of high energy phonon modes ($P_4$ and $P_5$) showing temperature-dependent shift near $T_N$.

## V. ESTIMATION OF MAGNETIC EXCHANGE AND ANISOTROPY PARAMETERS

The set of microscopic parameters reported in Ref. [S3] is used in Eqs. (5)-(9) of the main manuscript, and the theoretical magnetic field dependence for all three field orientations is shown in Fig. S6 by solid lines. Although the zero-field magnon gap energies are different, the magnetic field dependencies of the magnon modes roughly distinguish the magnetic axes for the in-plane configurations presented in Fig. 3 and Fig. 4 of the main manuscript. The bare magnon mode energies obtained after decoupling with the phonon modes are also shown in the respective plots (open symbols).

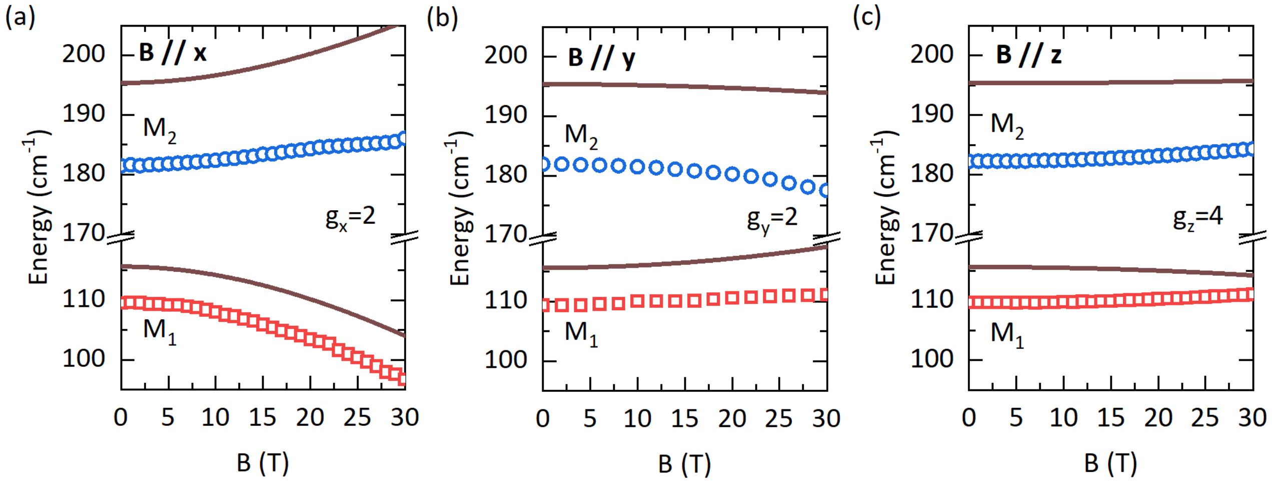


FIG. S6. (a)-(c) The theoretical evaluation of magnon modes ($M_1$, $M_2$) as a function of magnetic field applied along magnetic $x$-, $y$-, and $z$-axes respectively (solid lines). The exchange and anisotropy parameters are considered from Ref. [S3]: $J_{\rm eff}$ = 7.99 meV, $D$ = 6.07 meV, $E$ = -0.77 meV, $g_x$ = 2, $g_y$ = 2, and $g_z$ = 4. The bare magnon mode energies obtained for the configurations, presented in Figs. 3a and 4a of the main manuscript, are also shown in the respective plots (open symbols).

Since the in-plane magnetic field was applied at an arbitrary orientation, we opted to use the out-of-plane configuration ($B \parallel z$-axis) to estimate the microscopic magnetic parameters. Here we assume that the magnetic field remains perpendicular to the spin direction (even though it is canted by 10° out-of-plane). We used Eq. 4 of the main manuscript for the magnon gaps:

$$\omega_{M_1} = 2S\sqrt{(-2E)(J_{\rm eff}+D-E)}\ , \qquad \omega_{M_2} = 2S\sqrt{(D-E)(J_{\rm eff}-2E)}\ , \tag{S2}$$

and the slopes of the linear dependencies of $\omega^2_{M1}$ and $\omega^2_{M2}$ on $B^2$, as derived from **Eq. 5** of the main manuscript:

$$slope\ (M_1) = \left[\frac{2E}{(J_{eff}+D-E)}\right](g_z\mu_B)^2 \qquad slope\ (M_2) = \left[\frac{(J_{eff}-2E)(J_{eff}-D+E)}{(J_{eff}+D-E)^2}\right](g_z\mu_B)^2 \tag{S3}$$

The anisotropy parameter $E$ must be negative to yield a real value for the $M_1$ mode energy from Eq. S2. Consequently, the slope of $M_1^2$ versus $B^2$ is expected to be negative from Eq. S3, while that of $M_2^2$ should be positive. Experimentally, however, both $M_1$ and $M_2$ exhibit positive slopes, as shown in Fig. S3. The unexpected positive slope of the $M_1$ mode may result from an additional mixing term $K$ and a corresponding spin tilt within the $ac$-plane, as discussed in the main manuscript. Although the additional anisotropy term may also influence the field dependence of the $M_2$ mode, we assume it remains unaffected for the present analysis. We therefore use Eq. S2 and *slope* ($M_2$) from Eq. S3 to estimate the exchange and anisotropy parameters. The graphical solution is presented in Fig. S7a for $g_z = 4$ and the parameters are estimated to be $J_{eff} = 9.9$ meV, $D = 4.3$ meV, and $E = -0.7$ meV. These values are consistent with previously reported results[S3], with slight deviations attributed to differences in the bare magnon mode energies used in the analysis. On the other hand, $g_z = 2$ requires a very high value of $J_{eff}$ ($J_{eff} \gg D, E$) which

is neither consistent with reported value [S3] nor consistent with the Néel temperature ($J_{eff} = 3k_BT_N/S(S+1) =$ 8.3 meV for $J_{eff} \gg D, E$ ) [S4] and thus excluded. The same set of exchange and anisotropy parameters is used to simulate the magnetic field dependence of the magnon modes for $B \parallel x$ using **Eq. 9**, and for $B \parallel y$ using **Eq. 7** of the main manuscript, considering the g factor to be either 2 or 4. The resulting simulations are shown in Fig. S6b and Fig. S6c, respectively. The magnetic field dependence for the $B \parallel x$ configuration is best described by the simulation with $g_x = 2$. The interpretation of the magnetic field dependence along the $y$-axis is more complex, as the best fit is obtained with $g_y = 4$ for the $M_2$ mode and $g_y = 2$ for the $M_1$ mode. This inconsistency highlights limitations in our simplified model where the magnetic field dependence is known only along three orthogonal axes. It also assumes a symmetric effective exchange interaction and neglects the mixing term $K$. Despite this, the estimated exchange and anisotropy parameters are in good agreement with those obtained from neutron inelastic scattering experiments [S3]. Furthermore, our results provide experimental evidence supporting the presence of an anisotropic $g$-factor in $CoPS_3$.

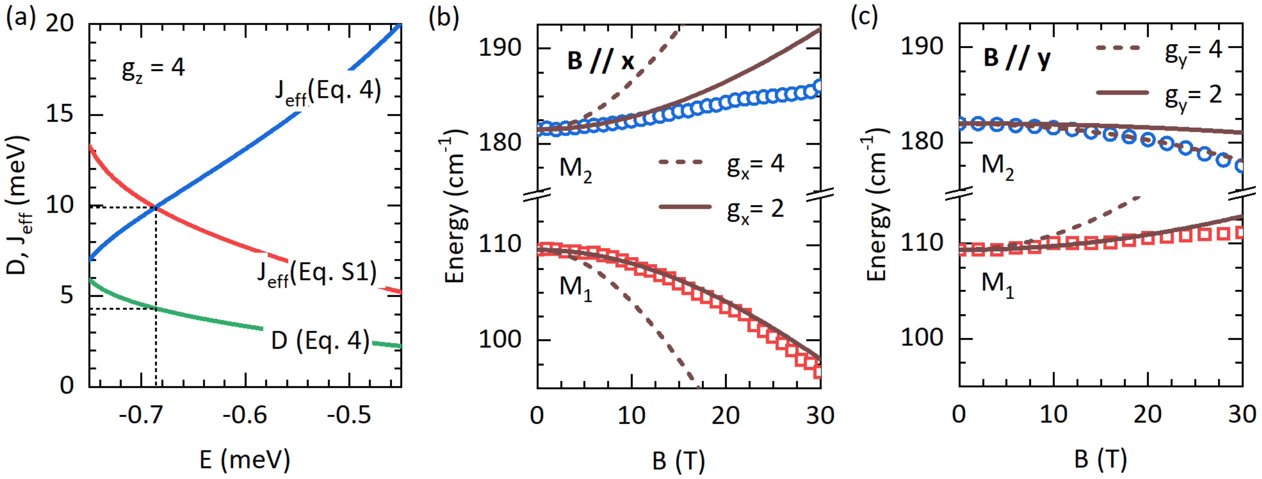


FIG. S7. (a) Graphical solution of **Eq. 4** of the main manuscript and and Eq. S3 for $M_2$ with $g_z = 4$. The vertical dashed line highlights the solution: $E = -0.7$ meV, while the horizontal dashed lines highlight the solution: $J_{eff} = 9.9$ meV, $D = 4.3$ meV. The simulated magnetic field dependence of the magnon modes for (b) $B \parallel x-axis$ and (c) $B \parallel y-axis$ configuration with the estimated exchange and anisotropy parameters and for the g-factor of 2 (solid lines) and 4 (dashed lines). The bare magnon energies as a function of magnetic field are also plotted in the respective figures.

[S1] Q. Liu, L. Wang, Y. Fu, X. Zhang, L. Huang, H. Su, J. Lin, X. Chen, D. Yu, X. Cui, J.-W. Mei, and J.-F. Dai, Magnetic order in XY-type antiferromagnetic monolayer $CoPS_3$ revealed by Raman spectroscopy, Phys. Rev. B **103**, 235411 (2021).
[S2] A. R. Wildes, V. Simonet, E. Ressouche, R. Ballou, and G. J. McIntyre, The magnetic properties and structure of the quasi-two-dimensional antiferromagnet $CoPS_3$, Journal of Physics: Condensed Matter **29**, 455801 (2017).
[S3] A. R. Wildes, B. Fåk, U. B. Hansen, M. Enderle, J. R. Stewart, L. Testa, H. M. Rønnow, C. Kim, and J.-G. Park, Spin wave spectra of single crystal $CoPS_3$, Phys. Rev. B **107**, 054438 (2023).
[S4] R. Basnet, K. M. Kotur, M. Rybak, C. Stephenson, S. Bishop, C. Autieri, M. Birowska, and J. Hu, Controlling magnetic exchange and anisotropy by nonmagnetic ligand substitution in layered $MPX_3$ ($M = Ni, Mn$; $X = S, Se$), Phys. Rev. Research **4**, 023256 (2022).
